# Supplementary material for: LightStereo: Channel Boost Is All You Need for Efficient 2D Cost Aggregation
Source: arXiv:2406.19833 source file (2025-02-26)
Supplement: Supplementary file 1 [file 7appendix.tex]

\section*{APPENDIX}

\section*{ACKNOWLEDGMENT}

This work was supported by the National Natural Science Foundation of China under Grant 62373356 and the Open Projects Program of the State Key Laboratory of Multimodal Artificial Intelligence Systems.
